# Supplementary material for: Variational r-Adaptive Cloth Simulation
Source: arXiv:2608.17833 source file (2026-08-18)
Supplement: Supplementary file 1 [file 08-appendix.tex]

\section{Cloth Elasticity Derivatives}
\label{app:derivatives}
Following~\cite{Wen:2023:KLS} and assuming the rest shape is completely flat (mean curvature $H=0$ and Gauss curvature $K=0$ everywhere), the elasticity per triangle $\triangle ijk$:
\begin{equation}
E_{ijk}=\frac{1}{2}hA_{ijk}\psi
\end{equation}
where
\begin{equation}
\begin{aligned}
\psi&= \psi(C_1)+\psi(C_2)\\
C_1&= F_0+\frac{\sqrt{3}}{6}hF_1,\quad C_2=F_0-\frac{\sqrt{3}}{6}hF_1\\
F_0&=tT^{-1}, \quad F_1=qT^{-1}\\
t&=\begin{bmatrix}x_j-x_i & x_k-x_i & n_{ijk} \end{bmatrix}\\
q&=2\begin{bmatrix}n_i-n_j & n_i-n_k & 0 \end{bmatrix}\\
T&=\begin{bmatrix}u_j-u_i & u_k-u_i & 0\\ 0 & 0& 1 \end{bmatrix}\\
\end{aligned}
\end{equation}

Here, $n$ is the mid-edge normal. Regarding the gradient,
\begin{equation}
\begin{aligned}
\frac{\partial E}{\partial x}&=\frac{1}{2}hA\frac{\partial \psi}{\partial x}\\
\frac{\partial E}{\partial u}&=\frac{1}{2}h(\frac{\partial A}{\partial u}\psi + A\frac{\partial \psi}{\partial u})
\end{aligned}
\end{equation}

where 
\begin{equation}
\begin{aligned}
\frac{\partial \psi}{\partial x} &= (\frac{\partial \psi_1}{\partial C_1}+\frac{\partial \psi_2}{\partial C_2})\frac{\partial F_0}{\partial t}\frac{\partial t}{\partial x}+\frac{\sqrt 3 h}{6}(\frac{\partial \psi_1}{\partial C_1}-\frac{\partial \psi_2}{\partial C_2})\frac{\partial F_1}{\partial q}\frac{\partial q}{\partial x}\\
\frac{\partial \psi}{\partial u}&=(\frac{\partial \psi_1}{\partial C_1}+\frac{\partial \psi_2}{\partial C_2})\frac{\partial F_0}{\partial T}\frac{\partial T}{\partial u}+\frac{\sqrt3h}{6}(\frac{\partial \psi_1}{\partial C_1}-\frac{\partial \psi_2}{\partial C_2})\frac{\partial F_1}{\partial T}\frac{\partial T}{\partial u}
\end{aligned}
\end{equation}

Regarding the Hessian,
\begin{equation}
\begin{aligned}
\frac{\partial^2 E}{\partial x^2} &= \frac{1}{2}hA\frac{\partial^2 \psi}{\partial x^2} \\
\frac{\partial^2 E}{\partial u^2} &=\frac{1}{2}h(\frac{\partial^2 A}{\partial u^2}\psi + \frac{\partial A}{\partial u}\frac{\partial \psi}{\partial u}^T + \frac{\partial \psi}{\partial u}\frac{\partial A}{\partial u}^T + A\frac{\partial^2 \psi}{\partial u^2} ) \\
\frac{\partial^2 E}{\partial x \partial u} &=\frac{1}{2}h (\frac{\partial \psi}{\partial x} \frac{\partial A}{\partial u}^T + A\frac{\partial^2 \psi}{\partial x \partial u} )
\end{aligned}
\end{equation}

where
\begin{equation}
\begin{aligned}
\frac{\partial^2 \psi}{\partial x^2} &= (\frac{\partial^2 \psi_1}{\partial C_1^2}\frac{\partial C_1}{\partial x}+\frac{\partial^2 \psi_2}{\partial C_2^2}\frac{\partial C_2}{\partial x})\frac{\partial F_0}{\partial t}\frac{\partial t}{\partial x}\\&+(\frac{\partial \psi_1}{\partial C_1}+\frac{\partial \psi_2}{\partial C_2})\frac{\partial F_0}{\partial t}\frac{\partial^2 t}{\partial x^2}\\
&+\frac{\sqrt3h}{6}(\frac{\partial^2 \psi_1}{\partial C_1^2}\frac{\partial C_1}{\partial x}-\frac{\partial^2 \psi_2}{\partial C_2^2}\frac{\partial C_2}{\partial x})\frac{\partial F_1}{\partial q}\frac{\partial q}{\partial x} \\&+\frac{\sqrt3h}{6} (\frac{\partial \psi_1}{\partial C_1}-\frac{\partial \psi_2}{\partial C_2}) \frac{\partial F_1}{\partial q} \frac{\partial^2 q}{\partial x^2}
\end{aligned}
\end{equation}

\begin{equation}
\begin{aligned}
\frac{\partial^2 \psi}{\partial u^2}&=(\frac{\partial^2 \psi_1}{\partial C_1^2}\frac{\partial C_1}{\partial u}+\frac{\partial^2 \psi_2}{\partial C_2^2}\frac{\partial C_2}{\partial u})\frac{\partial F_0}{\partial u}\\&+(\frac{\partial \psi_1}{\partial C_1}+\frac{\partial \psi_2}{\partial C_2})\frac{F_0}{\partial T^{-1}}\frac{\partial T}{\partial u}^T\frac{\partial^2 T^{-1}}{\partial T^2}\frac{\partial T}{\partial u}\\
&+\frac{\sqrt3h}{6}(\frac{\partial^2 \psi_1}{\partial C_1^2}\frac{\partial C_1}{\partial u}-\frac{\partial^2 \psi_2}{\partial C_2^2}\frac{\partial C_2}{\partial u})\frac{\partial F_1}{\partial u}\\&+\frac{\sqrt3h}{6}(\frac{\partial \psi_1}{\partial C_1}-\frac{\partial \psi_2}{\partial C_2})\frac{\partial F_1}{\partial T^{-1}}\frac{\partial T}{\partial u}^T\frac{\partial^2 T^{-1}}{\partial T^2}\frac{\partial T}{\partial u}
\end{aligned}
\end{equation}

\begin{equation}
\begin{aligned}
\frac{\partial^2 \psi}{\partial x\partial u}&=(\frac{\partial^2 \psi_1}{\partial C_1^2}\frac{\partial C_1}{\partial u} + \frac{\partial^2 \psi_2}{\partial C_2^2}\frac{\partial C_2}{\partial u}) \frac{\partial F_0}{\partial x}\\&+(\frac{\partial \psi_1}{\partial C_1}+\frac{\partial \psi_2}{\partial C_2})\frac{\partial t}{\partial x}^T\frac{\partial^2 F_0}{\partial t\partial T^{-1}}\frac{\partial T^{-1}}{\partial u} \\
&+\frac{\sqrt3h}{6}(\frac{\partial^2 \psi_1}{\partial C_1^2}\frac{\partial C_1}{\partial u} - \frac{\partial^2 \psi_2}{\partial C_2^2}\frac{\partial C_2}{\partial u})\frac{\partial F_1}{\partial x} \\&+\frac{\sqrt3h}{6}(\frac{\partial \psi_1}{\partial C_1}-\frac{\partial \psi_2}{\partial C_2}) \frac{\partial q}{\partial x}^T \frac{\partial^2 F_1}{\partial q \partial T^{-1}}\frac{\partial T^{-1}}{\partial u} 
\end{aligned}
\end{equation}
